# Supplementary material for: Data-driven learning of non-autonomous systems
Source: arXiv:2006.02392 source file (2020-06-02)
Supplement: Supplementary file 1 [file Appendix.tex]

\appendix
\section{Examples for local parameterization functions}
\label{sec:app1}
\begin{example}
	Taylor polynomials of degree $k$ at $t=t_n$, 
	\begin{equation}
	\label{eq:taylor}
	\tgamma_n(\tau; \ggamma_n)=\sum_{j=0}^k \hgamma^n_j\, \tau^j
	\end{equation}
	where $\hgamma^n_j=\frac{\gamma^{(j)}(t_n)}{j!}$, for $j=0, 1, \ldots, k$. 
	%In this case the upper bound for the approximation error is
	%\begin{equation*}
	%\eta = \|\gamma^{(k+1)}(t)\|_{L^\infty([0, T])} \frac{\Delta^{k+1}}{(k+1)!}.
	%\end{equation*}
\end{example}

\begin{example}
	Interpolating polynomials at $k+1$ equally spaced points in $[t_n, t_{n+1}]$
	\begin{equation}
	\label{eq:interp}
	\tgamma_n(\tau;\ggamma_n)=\sum_{j=0}^k \hgamma_j^n l_j(\tau),
	\end{equation}
	where
	\begin{equation*}
	\l_j(\tau)=\prod_{\substack{i=0,\\ i\neq j}}^k \,\frac{k\tau-i\delta_n}{(j-i)\delta_n}, \quad j=0, 1, \ldots, k,
	\end{equation*}
	are the Lagrange basis. The parameters are point values on equally spaced points in $[t_n, t_{n+1}]$, i.e., $\hgamma_j^n=\gamma(t_n+j\delta_n/k)$, for $j=0, 1, 2, \ldots, k$.
	% and the approximation error is bounded by
	%\begin{equation*}
	%\eta=\|\gamma^{(k+1)}(t)\|_{L^\infty([0, T])} \frac{\Delta^{k+1}}{(k+1)!}.
	%\end{equation*}
\end{example}

\begin{example}
	The $L^2$ projection into the polynomial space $\mathbb{P}^k([t_n ,t_{n+1}])$. 
	\begin{equation}
		\tgamma_n(\tau;\ggamma_n)=\sum_{j=0}^k \hgamma_j^n \widehat{\phi}_j(\tau)
	\end{equation}
	where $$\widehat{\phi}_j(\tau)=\sqrt{\frac{2j+1}{\delta_n}} p_j\left(\frac{2}{\delta_n}\tau-1\right), \quad s\in [0, \delta_n]$$ 
	and $\{p_j\}_{j=0}^k$ are the Legendre polynomials on the reference interval $[-1, 1]$ defined by the following recursive relationship:
	\begin{equation}
		(j+1)p_{j+1}(x)=(2j+1)\, x\, p_j(x)-j\,p_{j-1}(x), \quad p_0(x)=1, \quad p_1(x)=x,
	\end{equation}
	for $x\in [-1, 1]$. The parameters $\{\gamma^n_j\}_{j=0}^k$ are defined by
	\begin{equation}
		\gamma_j^n=\int_{t_{n}}^{t_{n+1}} \gamma(t)\widehat{\phi}_j(t-t_n)\,dt
		=\sqrt{\frac{(2j+1)\delta_n}{4}} \int_{-1}^1 \gamma\left( \frac{\delta_n}{2} (s+1)+t_n\right) p_j(s)\,ds.
	\end{equation}
	%The normalizing constants $\{w_j\}_{j=0}^k$ are defined by $w_j=\sqrt{\frac{2j+1}{2}}$, so that $\widehat{\phi}_j$ is orthonormal on $[t_n, t_{n+1}]$. The parameter $\gamma^n_j$ are the moments against the Legendre basis.
\end{example}

\section{A Proof of Proposition \ref{prop:NN_error}}
\label{sec:app2}
\begin{proof}
	Let us define $\tPPs=\hI+\tpphi$ as the exact evolution operator \eqref{evo_mod} for the modified system, where $\hI$ is defined in \eqref{hatI}. Then for any $\z, \y\in \R^d$, and $(\llambda, \delta)\in \R^{n_b}\times \R$ we have
	\begin{align}
	\label{eq: B1}
	\nonumber
	\abs{\tN(\z, \llambda, \delta; \Theta^*)-{\tPPs}(\y, \llambda, \delta; \Theta^*)}
	&\leq \abs{\tN(\z, \llambda, \delta; \Theta^*)-\tPPs(\z, \llambda, \delta)}+\abs{\tPPs(\z, \llambda, \delta)-{\tPPs}(\y, \llambda, \delta)}\\\nonumber
	&=\abs{\N(\z, \ggamma, \delta; \Theta^*)-\tpphi(\z, \ggamma, \delta)}+\abs{\tPPs(\z, \llambda, \delta)-{\tPPs}(\y, \llambda, \delta)}\\
	&\leq \mathcal{E}+e^{L_1\delta}|\z-\y|
	\end{align}
	where in the last step we have used \eqref{eq:err_NN} and the classical result on the continuity of dynamical system with respect to the initial data; see \cite[p. 109]{stuart1998dynamical}.
	
	To proceed, let us further set $\tPPs_k(\cdot)=\tPPs(\cdot, \ggamma_k, \delta_k)$ and $\hPPsi_k(\cdot)=\tN(\cdot, \ggamma_k, \delta_k;\Theta^*)$. 
	Then for $t=\sum_{k=0}^{n-1} \delta_k$, by \eqref{evo_mod} and \eqref{eq:prediction}, the solution and the approximation at time $t$ can be represented as $n$ compositions of one-step evolution operators as below
	\begin{equation*}
		\tx(t)=\tPPs_{n-1}\circ \tPPs_{n-2} \circ \cdots \tPPs_0(\x_0),\quad 
		\hx(t)=\hPPsi_{n-1}\circ \hPPsi_{n-2} \circ \cdots \hPPsi_0(\x_0).
	\end{equation*}
	Then by applying \eqref{eq: B1} recursively, we have
	\begin{align*}
	&|\wh{\x}(t)-\tx(t)|\\
	= & \abs{\hPPsi_{n-1}\circ\hPPsi_{n-2}\circ \cdots \circ\hPPsi_{0}(\x_0)-{\tPPs}_{n-1}\circ {\tPPs}_{{n-2}}\circ \cdots \circ {\tPPs}_{0}(\x_0)}\\
	\leq & \mathcal{E}+e^{L_1\delta_{n-1}}\abs{\wh{\PPsi}_{n-2}\circ \cdots \circ\wh{\PPsi}_{0}(\x_0)- {\tPPs}_{{n-2}}\circ \cdots \circ {\tPPs}_{0}(\x_0)}\\
	\leq & \ldots\\
	\leq & \mathcal{E}\left(1+e^{L_1\delta_{n-1}}+e^{L_1(\delta_{n-1}+\delta_{n-2})}+\ldots+e^{L_1\sum_{i=1}^{n-1}\delta_i}\right)\\
	\leq & \mathcal{E}\left(1+e^{L_1\Delta}+e^{2L_1\Delta}+\ldots+e^{(n-1)L_1\Delta}\right)\\
	= & \frac{e^{nL_1\Delta}-1}{e^{L_1\Delta}-1}\,\mathcal{E}
	\end{align*}
	which implies the result \eqref{eq:approx_err}.

\end{proof}
